# Supplementary material for: Melting curves of ice polymorphs in the vicinity of the liquid-liquid critical point
Source: arXiv:2302.08540 ancillary file (2023-02-16)
Supplement: Supplementary file 1 [file Manuscript-SI.pdf]

# Supplemental material for: Melting curves of ice polymorphs in the vicinity of the liquid-liquid critical point

Pablo M. Piaggi*

*Department of Chemistry, Princeton University, Princeton, NJ 08544, USA*

Thomas E. Gartner III*

*School of Chemical and Biomolecular Engineering, Georgia Institute of Technology, Atlanta, Georgia 30318, USA*

Roberto Car

*Department of Chemistry, Princeton University, Princeton, NJ 08544, USA and Department of Physics, Princeton University, Princeton, NJ 08544, USA*

Pablo G. Debenedetti†

*Department of Chemical and Biological Engineering, Princeton University, Princeton, NJ 08544, USA*

(Dated: February 16, 2023)

# Abstract

**CONTENTS**


I. Biased coexistence simulations 2
A. Method 2
1. Order parameters 3
2. Bias potential 5
3. Estimation of the free energy 6
4. Chemical potentials and melting points 7
B. Results 7
C. Validation with standard coexistence simulations 11

II. Integration of the Clausius-Clapeyron equation 12
A. Method 12
B. Results 14

III. Melting curve of ice VI 20

IV. Melting curve of ice V for the TIP4P/Ice model 21

V. Experimental melting curves for light water 22

References 24


## I. BIASED COEXISTENCE SIMULATIONS

### A. Method

In the biased coexistence simulation we consider a system in which liquid water is in direct coexistence with an ice polymorph (see FIG. 2F of the main part for a coexistence configuration in the case of ice III). Taking inspiration from the interface pinning technique


* These authors contributed equally
† pdebene@princeton.edu

**TABLE I :** *Parameters used in the definition of the environment similarity collective variables for different ice polymorphs. $m$ is the number of environments, $r_c$ is the cutoff used in the definition of environments, $\sigma$ is the spread of Gaussians in Eq. (2), $\kappa$ is the threshold value of the order parameter that distinguishes liquid and solid environments, protons refers to the proton configuration, and neighbors is the atom types of neighbors.*

| Ice | $m$ | $r_c$ (nm) | $\sigma$ (nm) | $\kappa$ | protons | neighbors |
|---|---|---|---|---|---|---|
| III | 12 | 0.40 | 0.0675 | 0.763 | partially ordered | O |
| IV | 28 | 0.42 | 0.085 | 1.25 | disordered | O |
| V | 28 | 0.42 | 0.04 | 0.5 | disordered | O |
| XIII | 28 | 0.42 | 0.04 | 0.57 | ordered | O, H |

[1], we introduce a bias potential such that the number of ice-like molecules in the system reversibly increases and decreases by the number of molecules in one ice layer. The bias potential is constructed along collective variables, also called order parameters, that we describe below.

### 1. *Order parameters*

We consider the atomic environments within a prescribed cutoff $r_c$ of each water molecule in a given ice polymorph. The number $m$ of distinct environments is equal to the number of molecules in the basis of the crystal structure. The environments $X = \chi_1, ...., \chi_m$ are the starting point for the construction of the order parameter of each polymorph.

Environments are centered at oxygen atoms. Only oxygen atoms are considered as neighbors for proton-disordered ices III, IV, and V. Protons are not included in the environments in order for the proton configuration to form spontaneously during the simulation without any bias towards a particular configuration.[2] We remark that ice III is partially proton ordered and we treat it on the same footing as fully disordered ice IV and V. For proton-ordered ice XIII we consider both oxygen atoms and protons as neighbors. The number $m$ of distinct environments and the cutoff $r_c$ for each ice polymorph is summarized in TABLE I.

The environment similarity kernel[3, 4] is then used to compare the atomic environments

$\chi_l \in X$ with a generic environment $\chi$,

$$k_{\chi_l}(\chi) = \int \sum_{\alpha} \rho^{\alpha}_{\chi_l}(\mathbf{r}) \rho^{\alpha}_{\chi}(\mathbf{r}) \, d\mathbf{r} \tag{1}$$

where $\rho^{\alpha}_{\chi_l}(\mathbf{r})$ and $\rho^{\alpha}_{\chi}(\mathbf{r})$ are the atomic densities of species $\alpha$ corresponding to the environments $\chi_l$ and $\chi$, respectively. We also define the environments $\chi^{\alpha}_l$ and $\chi^{\alpha}$ as subsets of $\chi_l$ and $\chi$ limited to the species $\alpha$. If the densities are represented by sums of Gaussians centered at the neighbors' positions with spread $\sigma$, the kernel becomes:

$$k_{\chi_l}(\chi) = \frac{1}{n} \sum_{\alpha} \sum_{i \in \chi^{\alpha}_l} \sum_{j \in \chi^{\alpha}} \exp\left( -\frac{|\mathbf{r}^l_i - \mathbf{r}_j|^2}{4\sigma^2} \right) \tag{2}$$

where $n$ is the number of neighbors in the environment $\chi_l$, and $\mathbf{r}^l_i$ and $\mathbf{r}_j$ are the positions of the neighbors in environments $\chi^{\alpha}_l$ and $\chi^{\alpha}$, respectively. In Eq. (2) we have added a normalization such that $k_{\chi_l}(\chi_l) = 1$. The $m$ similarity kernels derived from Eq. (2) allow us to identify if a given environment is compatible with one of the environments of an ice polymorph. However, it is convenient to have a single similarity measure between a given environment and any of the $m$ reference environments of a polymorph, and thus we define the best-match kernel

$$k_X(\chi) = \max\{k_{\chi_l}(\chi) : \chi_l \in X\}, \tag{3}$$

that compares the environments $\chi$ with all the environments $X$ of a given polymorph. $k_X(\chi)$ as defined in Eq. (3) is not continuous and not differentiable, and cannot be used directly in enhanced sampling MD simulations. For this reason we use a smooth approximation to the maximum function,

$$k_X(\chi) = \frac{1}{\lambda} \log \left( \sum_{l=1}^{m} \exp(\lambda k_{\chi_l}) \right) \tag{4}$$

where $\lambda$ has to be set to a large value which in our simulations was $\lambda = 100$. Since there is one value of $k_X(\chi)$ per oxygen atom, any given bulk configuration has a distribution of this quantity. The spread of the Gaussians $\sigma$ in Eq. (2) can be chosen such that the overlap between the distributions of $k_X(\chi)$ in ice and water is minimized.

The similarity kernel defined in Eq. (3) provides a way to characterize the environments in a given configuration as being compatible with the environments in a given ice polymorph. For a system of $N$ water molecules there are $N$ oxygen-centered environments $\chi^1, \chi^2, ..., \chi^N$. We thus define a global order parameter $n_{ice}$ that represents the number of environments

consistent with an ice polymorph,

$$n_{ice} = \{\text{number of } \chi^i \ : \ k_X(\chi^i) > \kappa\}, \tag{5}$$

Here, $\kappa$ is a watershed between values of $k_X(\chi^i)$ consistent with the liquid and those consistent with the solid. Appropriate values of $\sigma$ and $\kappa$ for each ice polymorph are shown in TABLE I. The order parameter defined in Eq. (5) can be made continuous and differentiable using,

$$n_{ice} = \sum_{i=1}^{N} f(k_X(\chi^i)) \tag{6}$$

where $f$ is a switching function that is $\sim 0$ and $\sim 1$ for $k_X(\chi^i)$ values consistent with the liquid and the solid, respectively. In particular we choose:

$$f(y) = \begin{cases} 0 \quad \text{if} \quad y < 0 \\ y^2(3-2y) \quad \text{if} \quad 0 < y < 1 \\ 1 \quad \text{if} \quad y > 1 \end{cases}, \tag{7}$$

where $y = (k_X(\chi^i) - k_1)/(k_2 - k_1)$, and $k_1$ and $k_2$ can be chosen as the peaks of the liquid and ice distributions of $k_X(\chi^i)$, respectively.

### 2. *Bias potential*

We build a bias potential using the on-the-fly probability enhanced sampling (OPES) algorithm[5, 6] that is an evolution of the well-known metadynamics technique. [7] The bias potential is a function of $n_{ice}$ and targets a multiumbrella ensemble [5] that produces an approximately uniform distribution in an interval from $n_{ice}^{low}$ to $n_{ice}^{high}$. The limits of the interval are chosen as integer multiples of the number of molecules in a crystal layer, $\Delta n_{layer}$, i.e., $n_{ice}^{low} = N_l \Delta n_{layer}$ and $n_{ice}^{high} = (N_l + 1)\Delta n_{layer}$ with $N_l \in \mathbb{N}$. The functional form of the bias potential is

$$V(n_{ice}) = -\frac{1}{\beta}\left(\frac{1}{N_{\lambda'}}\sum_{\lambda'=1}^{N_{\lambda'}} e^{-(n_{ice}-n_{ice}^{\lambda'})^2/2\sigma'^2+\beta\Delta F'_{\lambda}}\right) \tag{8}$$

where $\beta$ is the inverse temperature and $n_{ice}^{\lambda'}$ are $N_{\lambda'}$ points uniformly spaced in the interval from $n_{ice}^{low}$ to $n_{ice}^{high}$. In the simulations, the spacing between $n_{ice}^{\lambda'}$ is one molecule. $\Delta F_{\lambda}$ is the difference in free energy between the unbiased system and the system with an umbrella

potential at $n_{ice}^{\lambda'}$, and can be determined iteratively as described in Ref. 6. Other methods, such as umbrella sampling or metadynamics, can be used instead of OPES to construct the bias potential. The values of $n_{ice}^{low}$ to $n_{ice}^{high}$ for each ice polymorph are summarized in TABLE II.

**TABLE II :** *For each ice polymorph we list the interval sampled in biased coexistence simulations ($n_{ice}^{low}$ and $n_{ice}^{high}$) and the total number of water molecules in the simulation box $N$.*

| Ice | $n_{ice}^{low}$ | $n_{ice}^{high}$ | N |
|---|---|---|---|
| III | 324 | 378 | 648 |
| IV - small | 128 | 192 | 256 |
| IV - large | 1024 | 1152 | 2048 |
| V | 320 | 380 | 672 |
| XIII | 320 | 380 | 672 |

The typical behavior of a simulation is as follows. After an initial transient during which a suitable bias potential is determined, the simulation samples reversibly the full targeted range of ice-like molecules. The biased simulation can be then continued as long as needed, providing the statistics on $n_{ice}$ required to estimate the difference in free energy between the ice polymorph and the liquid. For ice III, $n_{ice}$ as a function of simulation time is shown in FIG. 2A of the main part.

### *3. Estimation of the free energy*

Once the bias potential is converged, the equilibrium properties of the system can be calculated through the reweighting technique. In particular, the unbiased probability of observing an ice slab composed of $n_{ice}$ molecules is:

$$P(n_{ice}) = \langle \delta(n_{ice} - n_{ice}(\mathbf{R})) \rangle_0 \tag{9}$$

where $\delta$ is the Dirac delta function and $\langle \cdot \rangle_0$ denotes an average over the unbiased ensemble (e.g., NPT) and $n_{ice}(\mathbf{R})$ is the number of ice-like molecules in a configuration characterized by atomic coordinates $\mathbf{R}$. This probability can be computed from the biased simulations

using the formula:

$$P(n_{ice}) = \frac{\langle \delta(n_{ice} - n_{ice}(\mathbf{R}))e^{\beta V} \rangle_V}{\langle e^{\beta V} \rangle_V} \tag{10}$$

where $\langle \cdot \rangle_V$ is an average over the biased ensemble and $V$ is the bias potential. In practice, the application of Eq. (10) corresponds to constructing a histogram with weights $e^{\beta V}$. The free-energy surface for $n_{ice}$ is obtained simply by using the relation:

$$\Delta G(n_{ice}) = -\frac{1}{\beta} \log P(n_{ice}). \tag{11}$$

This procedure allowed us to calculate the free energy surfaces shown in FIG. 2B for ice III.

#### *4. Chemical potentials and melting points*

It can be shown[8] that the slope of $\Delta G(n_{ice})$ is the chemical potential difference between ice and liquid water. The slope of $\Delta G(n_{ice})$ is obtained by performing an error-weighted linear least-squares fit. The chemical potential difference between ice III and liquid water for different thermodynamic conditions is shown in FIG. 2C of the main part. Once the chemical potential differences are known, the melting points $T_m$ are calculated using the condition that $\mu_{liq \to ice}(T_m) = 0$ at constant pressure. $T_m$ can be easily obtained by an error-weighted linear least-squares fit of $\mu_{liq \to ice}$ vs. temperature.

### B. Results

The analysis of the biased coexistence simulations for ice III are shown in FIG. 2 of the main part. Here, we show corresponding results for ice IV, V, and XIII in FIG. SI-1, SI-2, SI-3, and SI-4. For ice IV, we ran simulation on systems with 256 and 2048 molecules. In FIG. 3 of the main part we show the melting points of the system with 256 molecules decreased by 7 K to take into account finite-size effects.

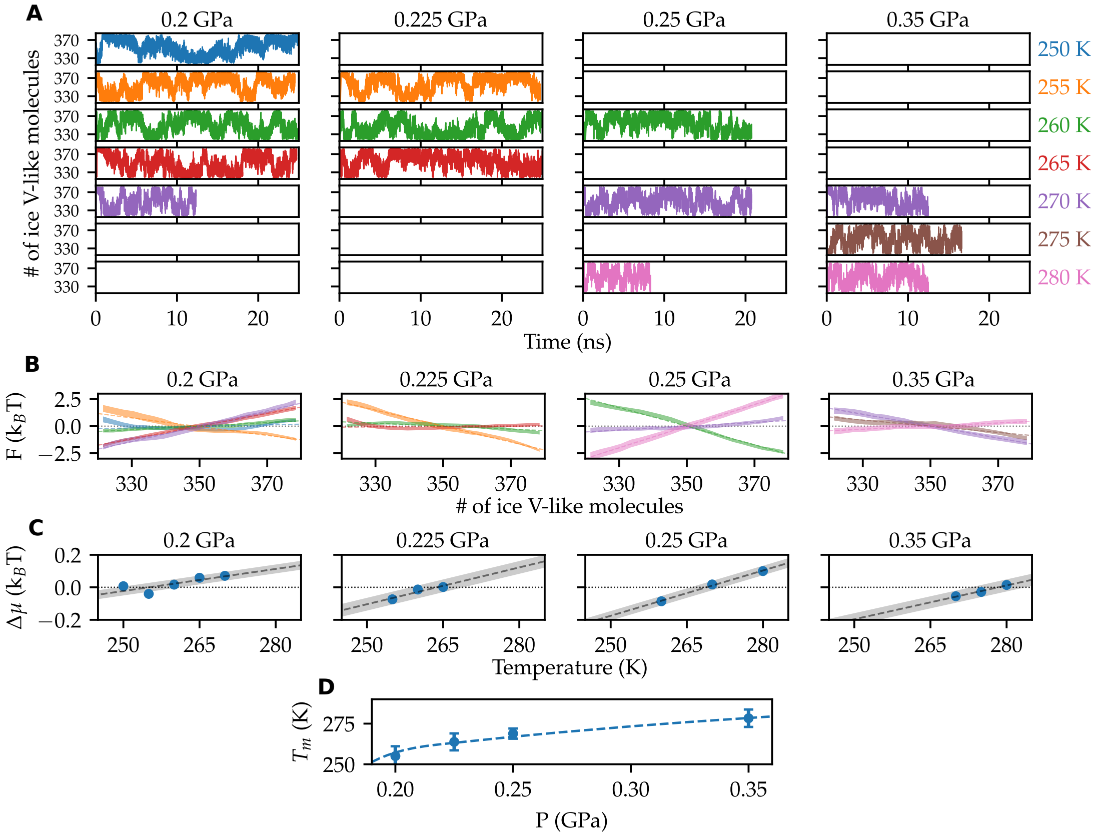


**FIG. SI-1 :** *Analysis of biased coexistence simulations for ice V. A) Number of ice-V like molecules vs time. B) Free energy surfaces as a function of the number of ice-V like molecules. C) Chemical potential vs temperature. The gray dashed line is a linear fit to the data, and the shaded region represents the one standard deviation errors in the fit parameters. D) Melting points of ice V. The dashed line is the melting curve obtained from the integration of the Clausius-Clapeyron equation.*

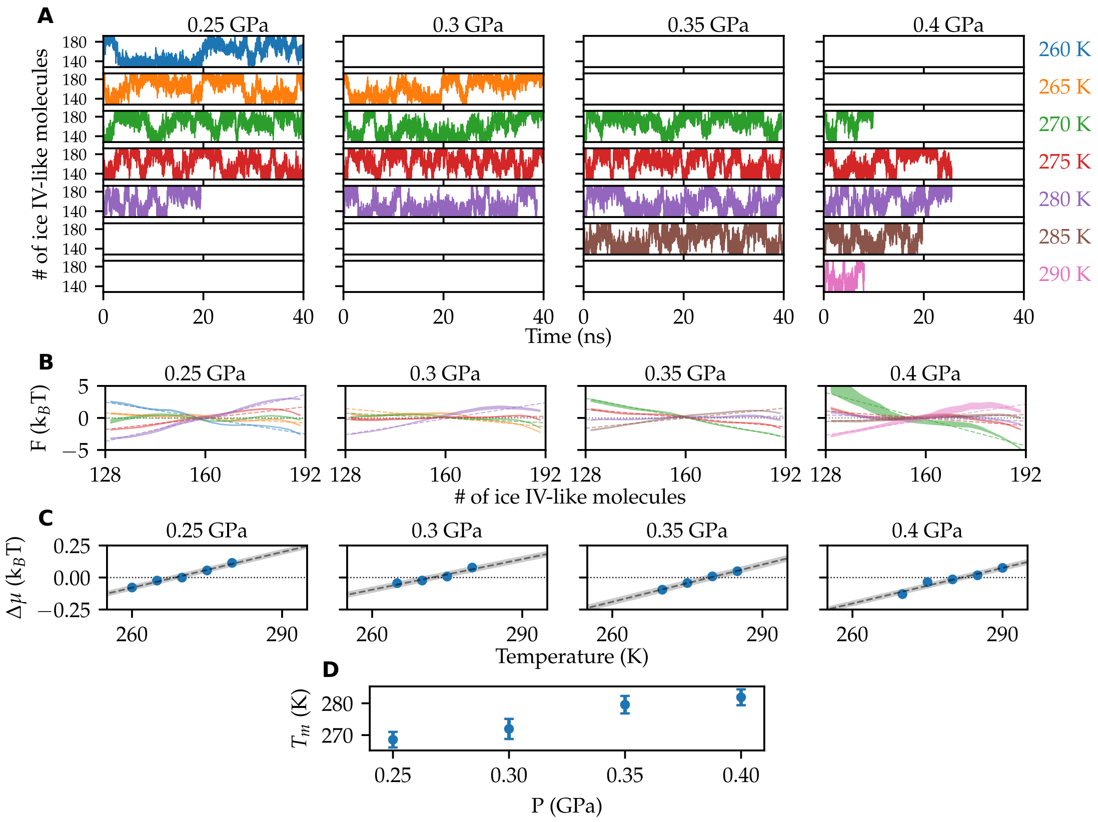


**FIG. SI-2 :** *Analysis of biased coexistence simulations for ice IV. The system used for these simulations contained 256 molecules. A) Number of ice-IV like molecules vs time. B) Free energy surfaces as a function of the number of ice-IV like molecules. C) Chemical potential vs temperature. The gray dashed line is a linear fit to the data, and the shaded region represents the one standard deviation errors in the fit parameters. D) Melting points of ice IV. These data have appreciable finite-size effects (compare with FIG. SI-3D).*

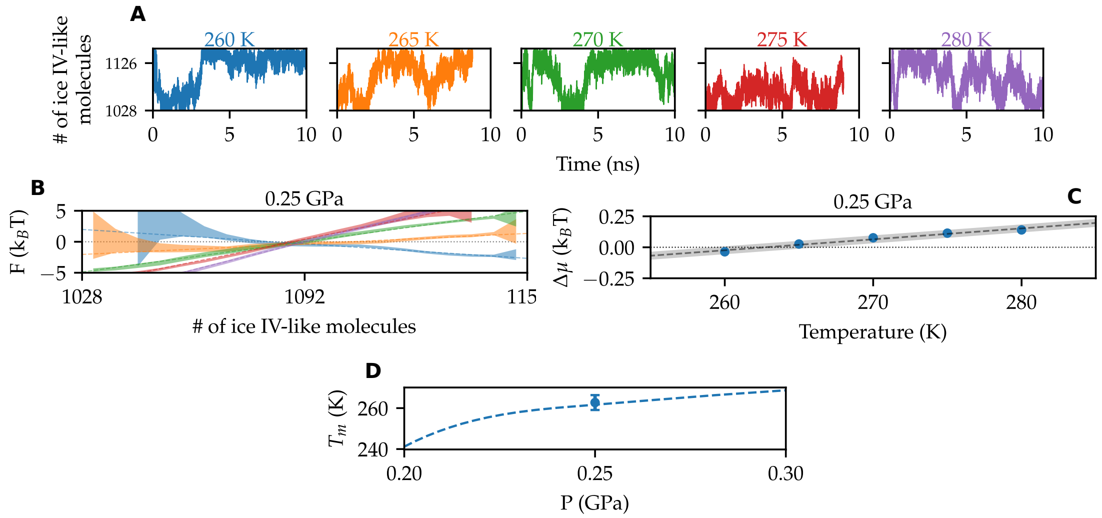


**FIG. SI-3 :** *Analysis of biased coexistence simulations for ice IV. The system used for these simulations contained 2048 molecules. A) Number of ice-IV like molecules vs time. B) Free energy surfaces as a function of the number of ice-IV like molecules. C) Chemical potential vs temperature. The gray dashed line is a linear fit to the data, and the shaded region represents the one standard deviation errors in the fit parameters. D) Melting points of ice IV. The dashed line is the melting curve obtained from the integration of the Clausius-Clapeyron equation.*

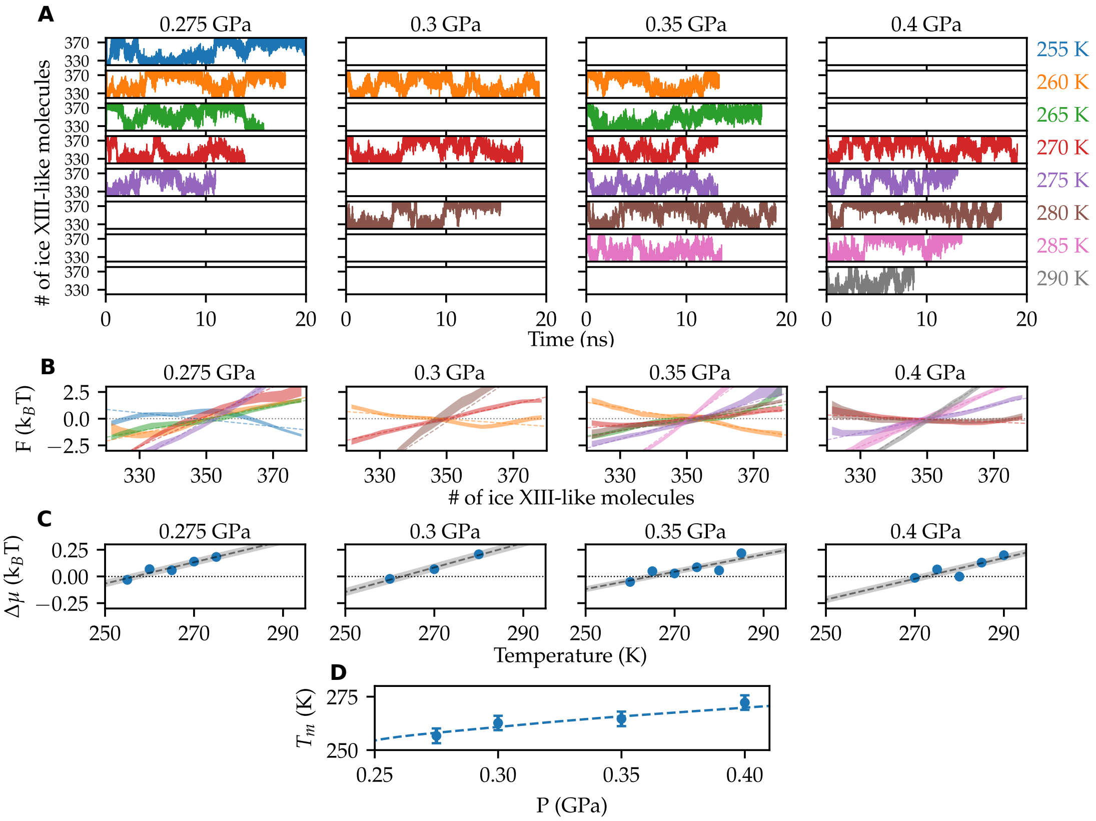


**FIG. SI-4 :** *Analysis of biased coexistence simulations for ice XIII. A) Number of ice-XIII like molecules vs time. B) Free energy surfaces as a function of the number of ice-XIII like molecules. C) Chemical potential vs temperature. The gray dashed line is a linear fit to the data, and the shaded region represents the one standard deviation errors in the fit parameters. D) Melting points of ice XIII. The dashed line is the melting curve obtained from the integration of the Clausius-Clapeyron equation.*

## C. Validation with standard coexistence simulations

We employed standard coexistence simulations as an additional method to validate our results for ice IV and V. We prepared configurations with ice and water in direct coexistence, and subsequently we ran them at different temperatures and pressures. The box sides parallel to the interface were fixed to the dimensions of the corresponding bulk ice crystal and the dimension perpendicular to the interface was barostatted to the desired pressure. The coexistence configurations employed for ice IV and V contained 2048 and 672 molecules, respectively. We controlled each simulation using the potential energy and visual inspection

in order to determine whether ice grew or melted. Below and above the melting temperature we expect ice to grow and melt, respectively, and from this information we can estimate the melting temperature. We summarize the results of our simulations in FIG. SI-5. The data shows very good agreement between all techniques that we used.

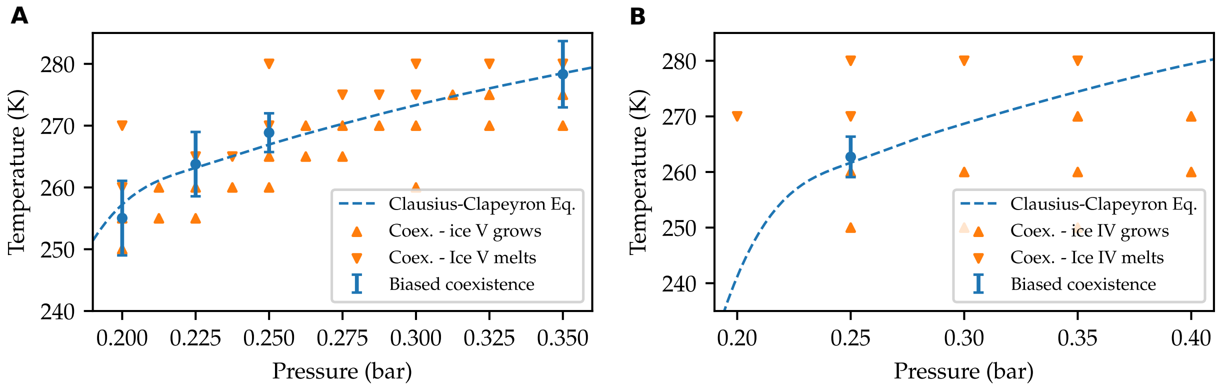


**FIG. SI-5 :** *Results of standard coexistence simulations. Comparison between different methods to calculate melting points of ice V (A) and ice IV (B). Up and down triangles represent state points at which ice in the configuration grew or melted, respectively. The circles and the error bars were obtained using biased coexistence simulations as described above. The dashed line was obtained by integration the Clausius-Clapeyron equation. All techniques are in good agreement with each other.*

## II. INTEGRATION OF THE CLAUSIUS-CLAPEYRON EQUATION

### A. Method

We calculated melting curves by integrating the Clausius-Clapeyron,

$$\frac{dT}{dP} = f(T,P) = \frac{T_m \, \Delta V}{\Delta H} \tag{12}$$

where $T_m$ is the melting temperature at pressure $P$, $\Delta V$ is the difference in molar volume between ice and liquid, and $\Delta H$ is the difference between ice and liquid. While the enthalpy and volume of ice polymorphs are easily computed from short ( 1 ns) simulation, the enthalpy and volume or the liquid require long simulation times, in particular at and below the Widom line. Thus, convergence of the properties of the liquid has to be carefully evaluated and we will discussed this point in detail below.

The integration is performed as follows. Starting from a known point of ice and liquid coexistence, $T_0$ and $P_0$, we employ a fourth-order Runge-Kutta integration scheme,

$$\begin{aligned} T_{n+1} &= T_n + \frac{1}{6}h(k_1 + 2k_2 + 2k_3 + k_4) \\ P_{n+1} &= P_n + h \end{aligned} \tag{13}$$

where $h$ is the pressure integration step that was set to 25 kPa and,

$$\begin{aligned} k_1 &= f(T_n, P_n) \\ k_2 &= f(T_n + h/2, P_n + h\, k_1/2) \\ k_3 &= f(T_n + h/2, P_n + h\, k_2/2) \\ k_4 &= f(T_n + h, P_n + h\, k_3). \end{aligned} \tag{14}$$

The starting points $T_0$ and $P_0$ were obtained from a linear fit to the coexistence points calculated via biased coexistence and are summarized in TABLE III. For ice VI we used a starting point from ref. 9.

**TABLE III :** *Starting points for the integration of the Clausius-Clapeyron equation to obtain the melting cruve for each polymorph. $T_0$ is the starting temperature and $P_0$ is the starting pressure.*

| Ice | $T_0$ (K) | $P_0$ (GPa) |
|---|---|---|
| III | 277.90 | 0.3 |
| IV | 261.65 | 0.25 |
| V | 273.33 | 0.3 |
| VI | 308.62 | 0.7 |
| XIII | 260.88 | 0.3 |

## B. Results

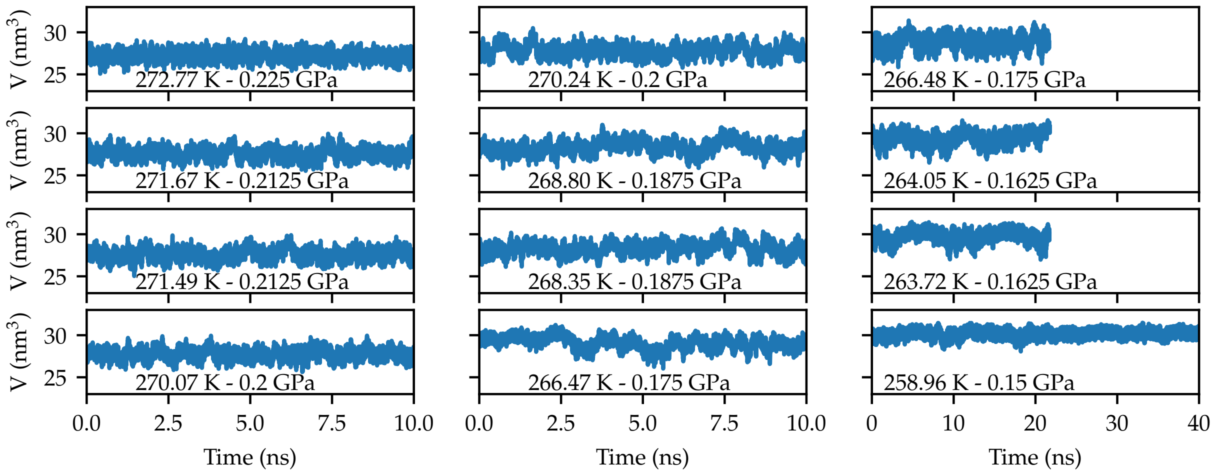


**FIG. SI-6 :** *Per-molecule volume of liquid water along the melting curve of ice III. These NPT trajectories were used to compute the enthalpy and volume needed in order to integrate the Clausius-Clapeyron equation.*

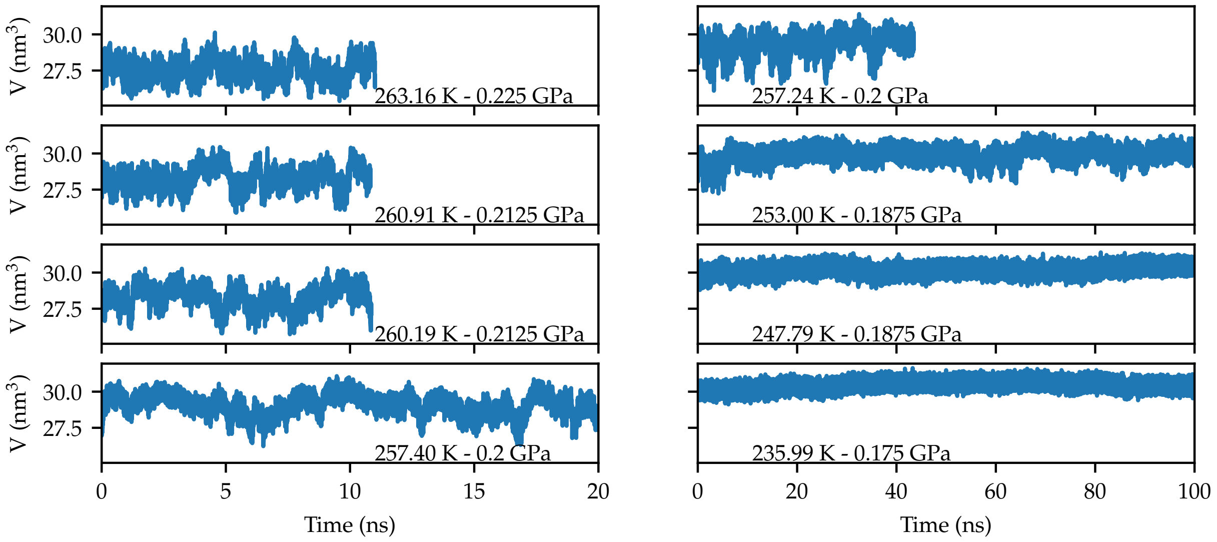


**FIG. SI-7 :** *Per-molecule volume of liquid water along the melting curve of ice V. These NPT trajectories were used to compute the enthalpy and volume needed in order to integrate the Clausius-Clapeyron equation.*

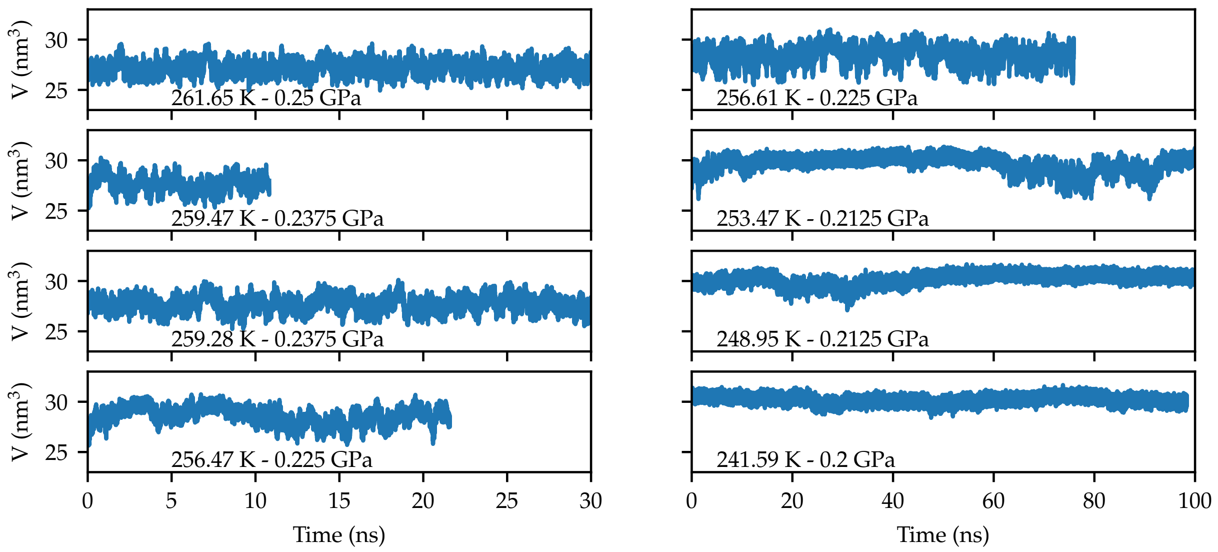


**FIG. SI-8 :** *Per-molecule volume of liquid water along the melting curve of ice IV. These NPT trajectories were used to compute the enthalpy and volume needed in order to integrate the Clausius-Clapeyron equation.*

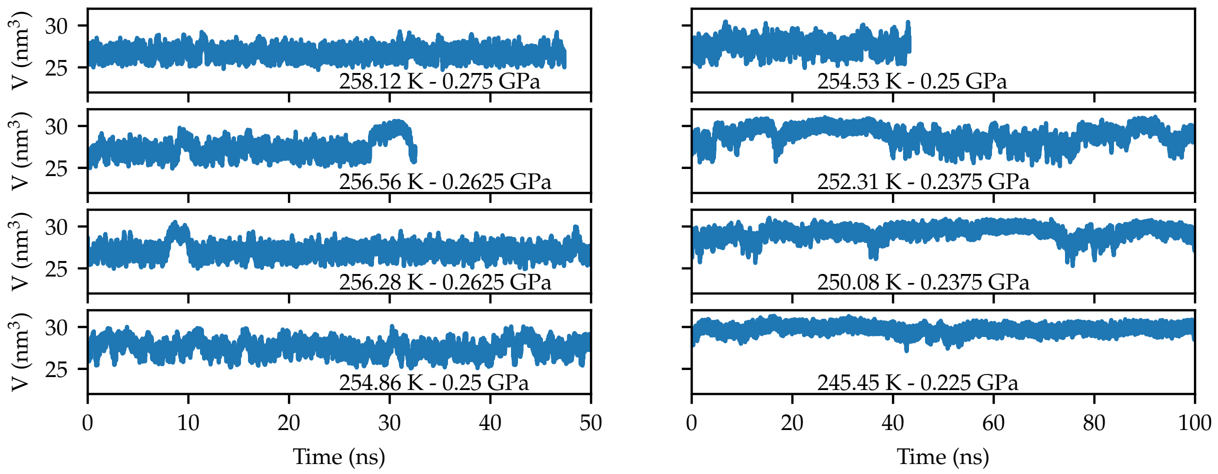


**FIG. SI-9 :** *Per-molecule volume of liquid water along the melting curve of ice XIII. These NPT trajectories were used to compute the enthalpy and volume needed in order to integrate the Clausius-Clapeyron equation.*

In FIG. SI-6, SI-7, SI-8, and SI-9 we show the per-molecule volume of liquid water as a function of simulation time for thermodynamic conditions along the melting lines of ice polymorphs. We used these simulations to compute the average volume needed in Eq. (12).

These figures illustrate the increase in correlation time as the coexistence line is traversed from HDL-like liquid to LDL-like liquid. In all cases, we evaluated the correlation times of the density to judge the appropriate length of the simulation. The enthalpy has a behavior similar to the volume and is not shown.

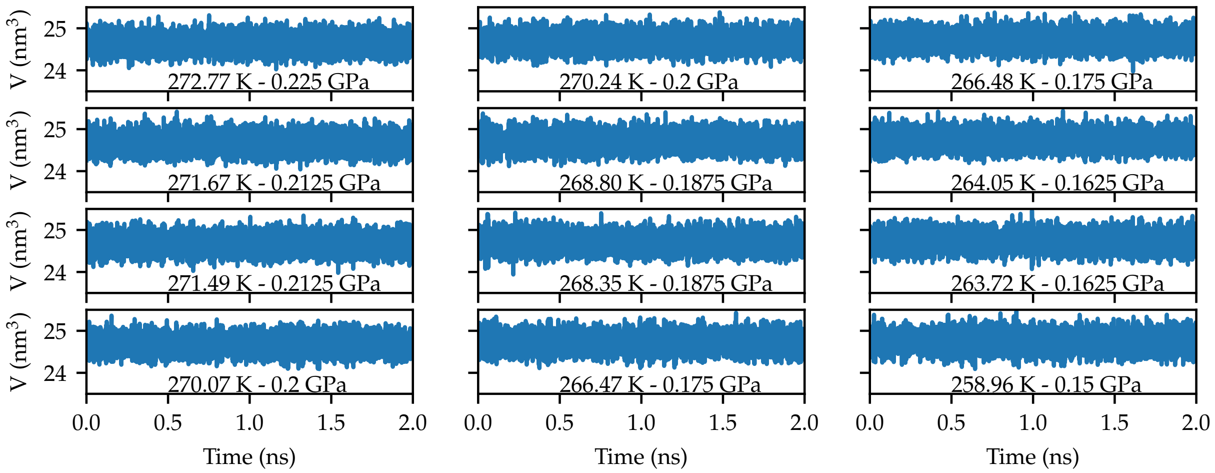


**FIG. SI-10 :** *Per-molecule volume of ice III along its melting curve. These NPT trajectories were used to compute the enthalpy and volume needed in order to integrate the Clausius-Clapeyron equation.*

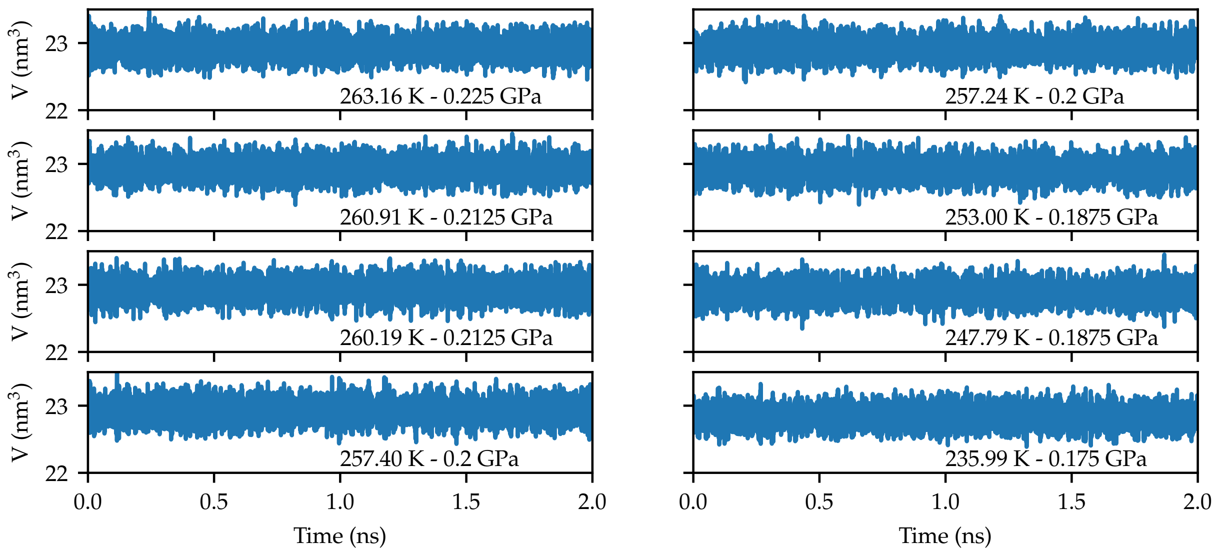


**FIG. SI-11 :** *Per-molecule volume of ice V along its melting curve. These NPT trajectories were used to compute the enthalpy and volume needed in order to integrate the Clausius-Clapeyron equation.*

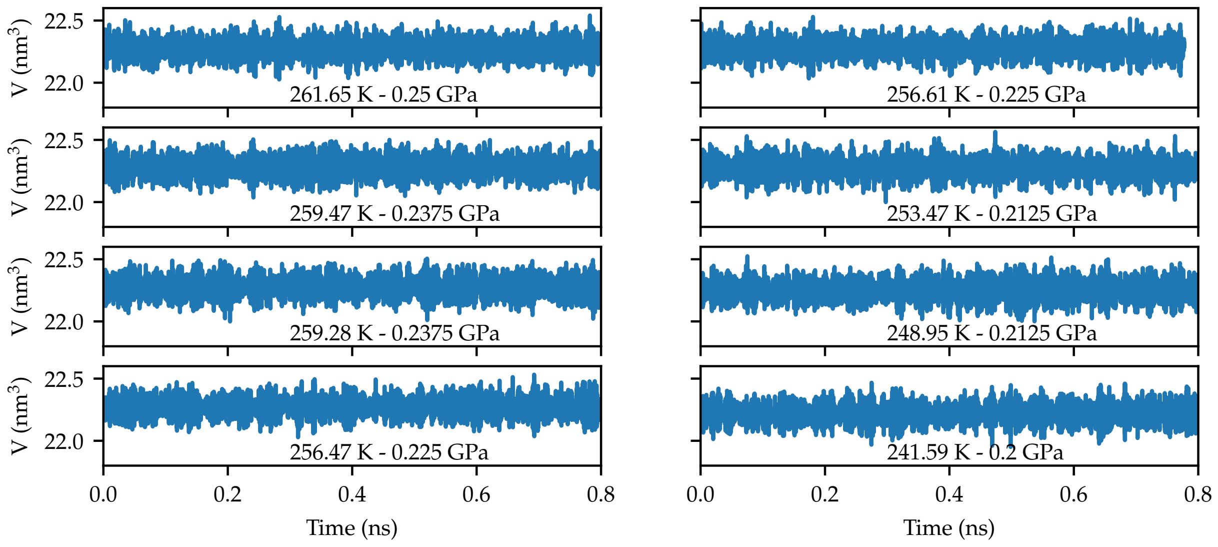


**FIG. SI-12 :** *Per-molecule volume of ice IV along its melting curve. These NPT trajectories were used to compute the enthalpy and volume needed in order to integrate the Clausius-Clapeyron equation.*

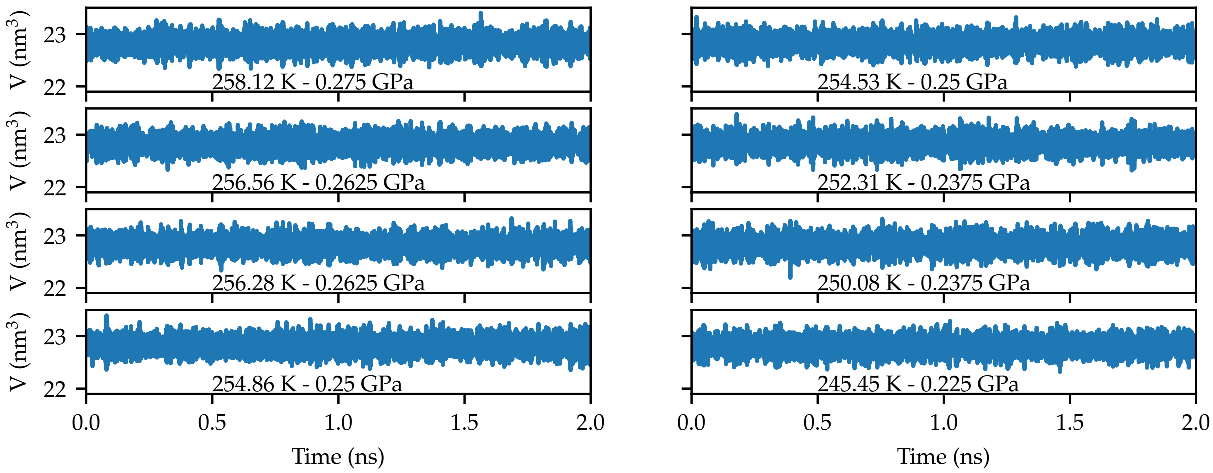


**FIG. SI-13 :** *Per-molecule volume of ice XIII along its melting curve. These NPT trajectories were used to compute the enthalpy and volume needed in order to integrate the Clausius-Clapeyron equation.*

In FIG. SI-10, SI-11, SI-12, and SI-13 we show the per-molecule volume of bulk ice polymorphs as a function of simulation time. Due to the short correlation time, simulations of ice polymorphs are significantly shorter than those of liquid water.

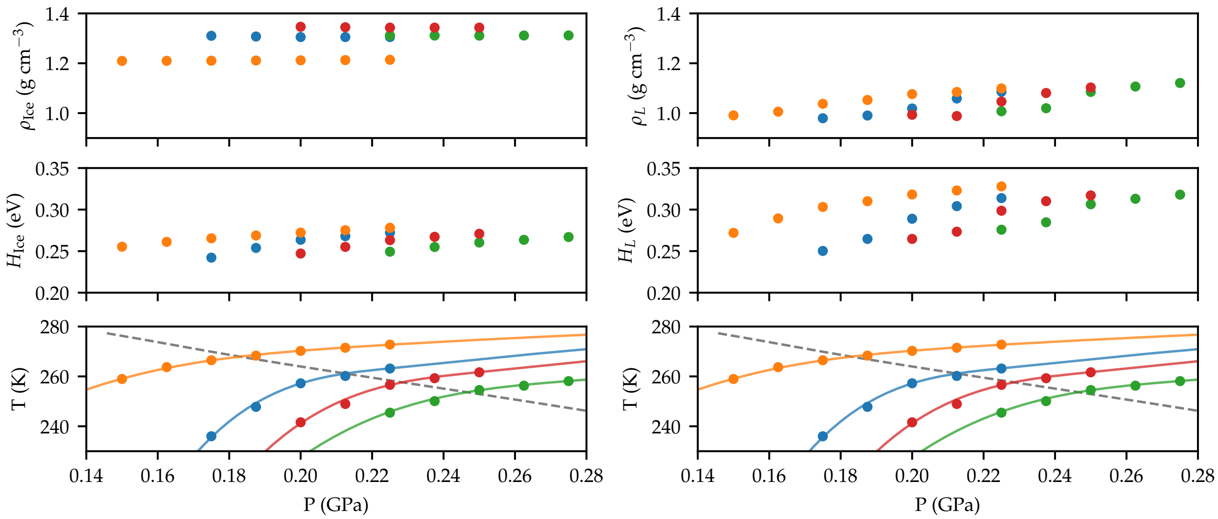


**FIG. SI-14 :** *Density $\rho_{\rm Ice}$ and enthalpy per molecule $H_{\rm Ice}$ of ices along melting lines of ice III (orange), V (blue), IV (red), and XIII (green). Density $\rho_L$ and enthalpy per molecule $H_L$ of liquid water along melting lines of ice III (orange), V (blue), IV (red), and XIII (green). Melting curves are shown below in order to characterize the thermodynamic state, temperature $T$ and pressure $P$, at which the properties were computed.*

In FIG. SI-14 we show the enthalpy and volume of ice polymorphs and we compare it to the same properties in liquid water. This figure shows that the changes in the properties of ices are much more subtle than the variations in the properties of liquid water. These changes are also analyzed in detail in TABLE IV.

**TABLE IV :** *Changes in the enthalpy and density of ice polymorphs and liquid water along melting curves. $T$ and $P$ are the temperature and pressure at selected points along the melting curves. $\rho_{\text{Ice}}$ and $H_{\text{Ice}}$ are the density and enthalpy of ice polymorphs, and $\rho_L$ and $H_L$ are the density and enthalpy of liquid water. We show data for two state points on the melting curve of each ice polymorph. We also provide percentage changes in the enthalpy and density.*

| Melting line | $T$ (K) | $P$ (GPa) | $\rho_{\text{Ice}}$ (g cm$^{-3}$) | $H_{\text{Ice}}$ (eV) | $\rho_L$ (g cm$^{-3}$) | $H_L$ (eV) |
|---|---|---|---|---|---|---|
| III-liquid | 272.77 | 0.225 | 1.214 | 0.278 | 1.099 | 0.328 |
| III-liquid | 258.96 | 0.150 | 1.209 | 0.255 | 0.991 | 0.272 |
| Change (%) | - | - | 0.41 | 8.3 | 9.8 | 17.1 |
| V-liquid | 263.16 | 0.225 | 1.305 | 0.272 | 1.086 | 0.314 |
| V-liquid | 235.99 | 0.175 | 1.310 | 0.242 | 0.979 | 0.250 |
| Change (%) | - | - | 0.4 | 11.0 | 9.9 | 20.4 |
| IV-liquid | 261.65 | 0.250 | 1.343 | 0.271 | 1.103 | 0.317 |
| IV-liquid | 241.59 | 0.200 | 1.346 | 0.247 | 0.993 | 0.265 |
| Change (%) | - | - | 0.2 | 8.9 | 10.0 | 16.4 |
| XIII-liquid | 258.12 | 0.275 | 1.312 | 0.267 | 1.121 | 0.318 |
| XIII-liquid | 245.45 | 0.225 | 1.312 | 0.249 | 1.006 | 0.276 |
| Change (%) | - | - | 0.0 | 6.7 | 10.3 | 13.2 |

## III. MELTING CURVE OF ICE VI

We show in FIG. SI-15 the melting curve of ice VI obtained by the integration of the Clausius-Clapeyron equation. We used the starting point $T$=308.62 K,$P$=0.7 GPa for the integration, as reported in ref. 9. The data shows that the melting curve of ice VI is supercritical. Furthermore, the relative position of the melting curve of ice VI with respect to the melting curves of other ice polymorphs is in excellent agreement with the experimental results of ref. [10].

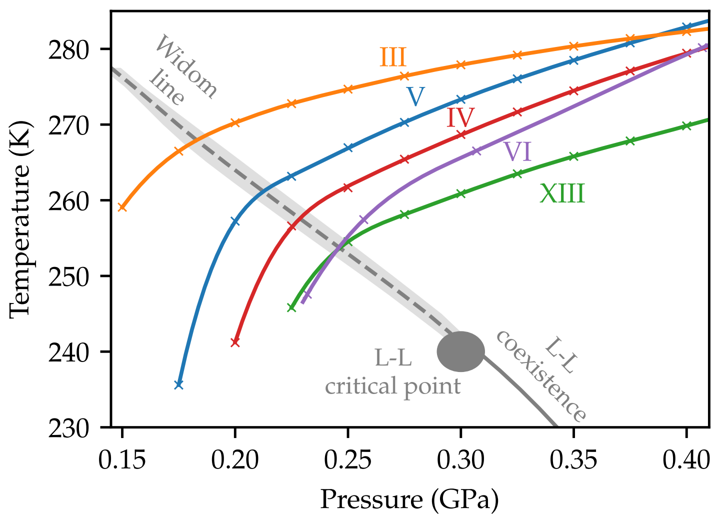


**FIG. SI-15 :** *Melting curves of ice polymorphs as predicted by our simulations based on the SCAN DFT functional. This figure closely follows FIG. 3 of the main text, and here we add the melting curve of ice VI that was not shown in FIG. 3 for clarity.*

## IV. MELTING CURVE OF ICE V FOR THE TIP4P/ICE MODEL

We calculated the melting curve of ice V in the TIP4P/Ice model by integrating the Clausius-Clapeyron equation. The starting point for the integration was the coexistence point $T$=241.1 K,$P$=0.4053 GPa from ref. .8. Each simulation used in the calculation of the enthalpy and volume required in Eq. 12 had a total length of 100 ns. The data shows that the melting curve of ice V within the TIP4P/Ice model is supercritical, in agreement with SCAN results shown in the main part of this work and in disagreement with the interpretation of experiments in ref. [10].

The computational details for the TIP4P/Ice[11] simulations are as follows. The MD simulations were carried out using LAMMPS[12, 13] and a time step of 2 fs for the integration of the equations of motion. The temperature was controlled using the stochastic velocity rescaling algorithm with a 0.1 ps relaxation time.[14] The pressure was maintained by the Parrinello-Rahman barostat with a 1 ps relaxation time.[15] The bond lengths and angles were kept fixed using the SHAKE algorithm. A cutoff of 0.85 nm was used for the Lennard-Jones and Coulomb interactions. Long-range Coulomb interactions beyond this cutoff were computed using the particle-particle particle-mesh (PPPM) solver with relative accuracy

$10^{-5}$. Tail corrections to the pressure and energy were included to take into account long-range effects neglected due to the Lennard-Jones potential truncation. The parameters for the Lennard-Jones interactions, charges, M-site position, and bond lengths were those reported in in ref. [11].

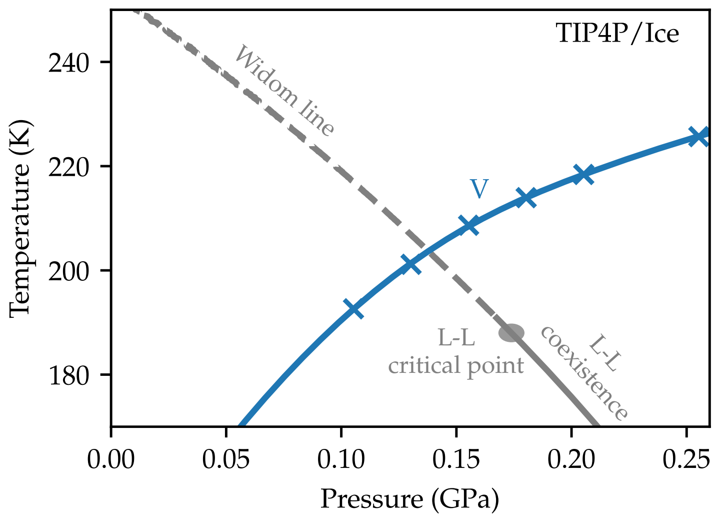


**FIG. SI-16 :** *Melting curve of ice V calculated with the TIP4P/Ice semiempirical water model. The location of the critical point for this model was obtained from ref. [16]. The liquid-liquid binodal and Widom line were obtained from a fit of the density and energy to a two-state equation of state (data provided by Jack Weis)[17].*

## V. EXPERIMENTAL MELTING CURVES FOR LIGHT WATER

In the main part of the manuscript we discussed the isotopic effects on the melting curves of ice polymorphs. In FIG. SI-17 we show the melting curves of light water ice polymorphs as reported in ref. 18. The relation between the melting curves and the location of the liquid-liquid critical point is similar to that shown in FIG. 3B of the main part for heavy water.

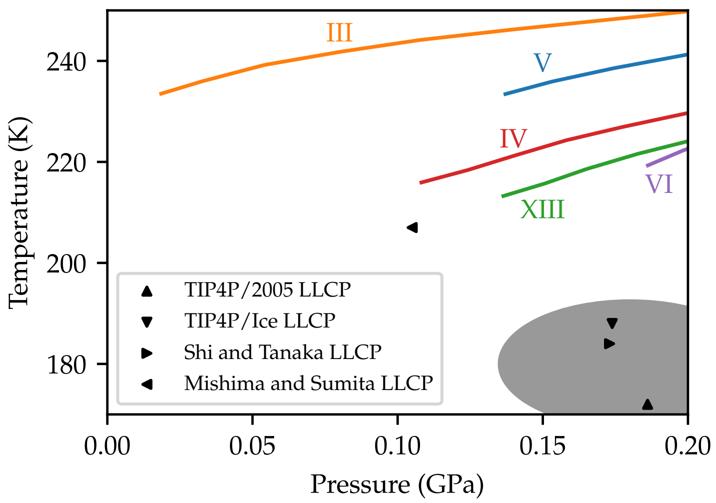


**FIG. SI-17 :** *Melting curves of ice polymorphs III, IV, V, VI, and XIII reported by Mishima [18] for light water. The shaded region is the location of the critical point estimated by Bachler et al. [19]. We also show the location of the critical point obtained by Shi and Tanaka using experimental measurements [20], by Debenedetti et al. using molecular simulations with the empirical water models TIP4P/2005 and TIP4P/Ice [16], and by Mishima and Sumita[21] using an extrapolation based on polynomial fits to equation of state data.*

[1] U. R. Pedersen, F. Hummel, G. Kresse, G. Kahl, and C. Dellago, Computing gibbs free energy differences by interface pinning, Phys. Rev. B **88**, 094101 (2013).

[2] P. M. Piaggi and R. Car, Phase equilibrium of liquid water and hexagonal ice from enhanced sampling molecular dynamics simulations, J. Chem. Phys. **152**, 204116 (2020).

[3] P. M. Piaggi and M. Parrinello, Calculation of phase diagrams in the multithermal-multibaric ensemble, J. Chem. Phys. **150**, 244119 (2019).

[4] A. P. Bartók, R. Kondor, and G. Csányi, On representing chemical environments, Phys. Rev. B **87**, 184115 (2013).

[5] M. Invernizzi, P. M. Piaggi, and M. Parrinello, Unified approach to enhanced sampling, Phys. Rev. X **10**, 041034 (2020).

[6] M. Invernizzi and M. Parrinello, Rethinking metadynamics: from bias potentials to probability distributions, J. Phys. Chem. Lett. **11**, 2731 (2020).

[7] A. Laio and M. Parrinello, Escaping free-energy minima, Proc. Natl. Acad. Sci. U.S.A. **99**, 12562 (2002).

[8] S. L. Bore, P. M. Piaggi, R. Car, and F. Paesani, Phase diagram of the tip4p/ice water model by enhanced sampling simulations, J. Chem. Phys. **157**, 054504 (2022).

[9] L. Zhang, H. Wang, R. Car, and W. E, Phase diagram of a deep potential water model, Phys. Rev. Lett. **126**, 236001 (2021).

[10] O. Mishima, Liquid-liquid critical point in heavy water, Phys. Rev. Lett. **85**, 334 (2000).

[11] J. Abascal, E. Sanz, R. García Fernández, and C. Vega, A potential model for the study of ices and amorphous water: Tip4p/ice, J. Chem. Phys. **122**, 234511 (2005).

[12] S. Plimpton, Fast parallel algorithms for short-range molecular dynamics, J. Comput. Phys. **117**, 1 (1995).

[13] A. P. Thompson, H. M. Aktulga, R. Berger, D. S. Bolintineanu, W. M. Brown, P. S. Crozier, P. J. in't Veld, A. Kohlmeyer, S. G. Moore, T. D. Nguyen, *et al.*, Lammps-a flexible simulation tool for particle-based materials modeling at the atomic, meso, and continuum scales, Comput. Phys. Commun. **271**, 108171 (2022).

[14] G. Bussi, D. Donadio, and M. Parrinello, Canonical sampling through velocity rescaling, J. Chem. Phys. **126**, 014101 (2007).

[15] M. Parrinello and A. Rahman, Polymorphic transitions in single crystals: A new molecular dynamics method, J. Appl. Phys. **52**, 7182 (1981).

[16] P. G. Debenedetti, F. Sciortino, and G. H. Zerze, Second critical point in two realistic models of water, Science **369**, 289 (2020).

[17] J. Weis, F. Sciortino, A. Z. Panagiotopoulos, and P. G. Debenedetti, Liquid–liquid criticality in the wail water model, J. Chem. Phys. **157**, 024502 (2022).

[18] O. Mishima, *Liquid-Phase Transition in Water* (Springer, 2021).

[19] J. Bachler, J. Giebelmann, and T. Loerting, Experimental evidence for glass polymorphism in vitrified water droplets, Proc. Natl. Acad. Sci. U.S.A. **118**, e2108194118 (2021).

[20] R. Shi and H. Tanaka, The anomalies and criticality of liquid water, Proc. Natl. Acad. Sci. U.S.A. **117**, 26591 (2020).

[21] O. Mishima and T. Sumita, Equation of state of liquid water written by simple experimental polynomials and the liquid–liquid critical point, J. Phys. Chem. B (2023).
